# Supplementary material for: Multi-Modal Fusion in Contact-Rich Precise Tasks via Hierarchical Policy Learning
Source: arXiv:2202.08401 source file (2022-02-17)
Supplement: Supplementary file 1 [file appendix.tex]

\section*{APPENDIX}
